# Supplementary material for: Isopignistic Canonical Decomposition via Belief Evolution Network
Source: arXiv:2405.02653 source file (2024-08-30)
Supplement: Supplementary file 1 [file suppley.tex]

\documentclass{article}

% Language setting
% Replace `english' with e.g. `spanish' to change the document language
\usepackage[english]{babel}

% Set page size and margins
% Replace `letterpaper' with`a4paper' for UK/EU standard size
\usepackage[letterpaper,top=2cm,bottom=2cm,left=3cm,right=3cm,marginparwidth=1.75cm]{geometry}

% Useful packages
\usepackage[utf8]{inputenc}
\usepackage{lineno}
\usepackage{array}
\usepackage{amssymb,amsthm}
\usepackage{enumerate}
\usepackage{makecell}
\usepackage{mathtools}
\usepackage{array}
\usepackage{multirow}
\usepackage{slashed}
\usepackage{ulem}
\usepackage{color}
\usepackage{diagbox}
\usepackage{enumerate}
\usepackage{graphicx}
\allowdisplaybreaks[1]
\usepackage{subfigure}
 \usepackage{tikz} 
\usepackage{indentfirst}
\usepackage{soul}
\usepackage{amsmath}
\usepackage[justification=centering]{caption}
\usepackage{tabularx}
\usepackage{algorithm}
\usepackage{algorithmic}
\usepackage{adjustbox}

\usetikzlibrary{shapes.geometric, arrows}
\modulolinenumbers[5]

\newtheorem{example}{Example}
\newtheorem{proposition}{Proposition}

\newcommand{\circledsmall}[1]{\hbox{\tikz\draw (0pt, 0pt)
    circle (.5em) node {\makebox[0.15em][c]{\scriptsize#1}};}}
\newcommand{\circledtiny}[1]{\hbox{\tikz\draw (0pt, 0pt)
    circle (.4em) node {\makebox[0.01em][c]{\tiny#1}};}}

\usepackage[colorlinks=true, allcolors=blue]{hyperref}

\title{Supplementary Material for \textbf{Isopignistic Canonical Decomposition via Belief Evolution Network}}
\author{Anonymous submission}

\begin{document}
\maketitle

\section{Proofs}

\subsection{Proposition \ref{p1}}
\begin{proposition}\label{p1}
    If a probability transformation method satisfies upper and lower bounds consistency, i.e., $p(\omega_i) \in [Bel({\omega_i}), Pl({\omega_i})]$, it can be implemented via the BEN.
\end{proposition}
\begin{proof}
    If the range of $\tau$ and $\xi$ is $[0,1]$, the $m_{\text{B}}(\{\omega_i\})\geq m(\{\omega_i\})=Bel(\{\omega_i\})$. In BEN, the receiving beliefs focal sets must be the subset of the transferring beliefs focal sets. Hence, for the $m_{\text{B}}(\{\omega_i\})$, its potential transferred beliefs should satisfy $m_{\text{B}}(\{\omega_i\})\leq \sum_{\omega_i\in F_j}m(F_j)=Pl(\{\omega_i\})$. Hence, BEN can implement probability transformation which satisfy the $p(\omega_i)\in[Bel(\{\omega_i\}),Pl(\{\omega_i\})]$.
\end{proof}
\subsection{Proposition \ref{p2}}
\begin{proposition}\label{p2}
    If the BEN adheres to the condition $\tau(F_i) = 1$ and $\xi(\frac{F_j}{F_i})=\frac{1}{|F_j|}$, then the outcome of applying the BEN to any BPA will coincide with its $BetP$, i.e., $BetP_{m}=T_{\mathfrak{B}}(m)$.
\end{proposition}
\begin{proof}
Consider the calculation of the PPT. For each $\omega \in F_i$, the belief $\frac{m(F_j)}{|F_j|}$ in $BetP(\omega)$ is contributed by $m(F_i)$. In BEN, since $\tau(F_i) = 1$ and $\xi(\frac{F_i}{F_j})=\frac{1}{|F_i|}$, all beliefs on $F_i$ will be transferred to its child nodes. Among them, belief $m(F_i)\times\frac{|F_j|}{|F_i|}$ is transferred to the focal sets that contain $\omega$. Continue in the same way, $m(F_i)\times\frac{|F_j|}{|F_i|}\times\frac{|F_j|-1}{|F_j|}\times\cdots\times\frac{1}{2}=\frac{m(F_j)}{|F_j|}$. Therefore, for $m(F_i)$, the belief contribution to element $\omega$ after performing BEN equals $\frac{m(F_j)}{|F_j|}$, which is the same as PPT. Hence, when BEN adheres to the above conditions, BEN's revision is coincide with PPT.
\end{proof}
\subsection{Proposition \ref{p3}}
\begin{proposition}[Role of $\zeta$]\label{p3}
Consider an isopignistic transformation $m_2 = T_{\mathfrak{IB}}(m_1)$. If its isotransformation function is $\zeta$, then $\zeta'$, satisfying $\zeta'(F_i) = -\zeta(F_i)$, will serve as the isotransformation function for the inverse transformation $m_1 = T_{\mathfrak{IB}'}(m_2)$.
\end{proposition}
\begin{proof}
For an isopignistic transformation, the subset $F_i$ requires two operations: receiving beliefs from parent nodes and sending beliefs to child nodes. 
Suppose that in the transformation performed by $\mathfrak{IB}$, $F_i$ will receive beliefs $F_i$ is $\sum_{F_i\subset F_k, |F_k|=|F_i|+1}\frac{\zeta(F_k)}{|F_k|}$, and send beliefs $\zeta(F_i)$, so the transformed outcome is $$m_2(F_i)=m_1(F_i)+\sum_{F_i\subset F_k, |F_k|=|F_i|+1}\frac{\zeta(F_k)}{|F_k|}-\zeta(F_i).$$
If perform the transformation using $-\zeta$, the outcome will be
$$m_2(F_i)+\zeta(F_i)-\sum_{F_i\subset F_k, |F_k|=|F_i|+1}\frac{\zeta(F_k)}{|F_k|}=m_1(F_i).$$ Therefore, when taking a negative value for $\zeta$, the inverse transformation can be achieved.
\end{proof}
\subsection{Proposition \ref{p4}}
\begin{proposition}[Role of $\tau$]\label{p4}
    If all values of $\tau$ lie within the range $[-1,1]$, for any BPA $m$, the outcome of the transformation $m'$ using $\mathfrak{IB}=\{\mathcal{G}_{\Omega},\tau\}$ remains a BPA. In other words, it adheres to the conditions $m'(F_i)\in[0,1]$ and $\sum_{F_i\subseteq \Omega}m'(F_i)=1$.
\end{proposition}
\begin{proof}
    In terms of the forward transfer, it should satisfy $\tau(F_i)>0$, and the corresponding revision is $$m'(F_i)=(1-\tau(F_i))\times m(F_i)$$ and $$m'(F_j)=m(F_j)+\frac{\tau(F_i)\times m(F_i)}{|F_i|}$$ when $F_j\subset F_i$ and $|F_j|=|F_i|-1$. Since the $\tau(F_i)\in(0,1]$, $m'$ satisfies that $m'(F_i)$ and $m'(F_j)$ locating in the $[0,1]$ and $$m(F_i)+\sum_{F_j\subset F_i;|F_j|=|F_i|-1}m(F_j)=m'(F_i)+\sum_{F_j\subset F_i;|F_j|=|F_i|-1}'m(F_j).$$ In terms of the backward transfer, it should satisfy $\tau(F_i)<0$, and the corresponding revision is $$m'(F_i)=-\tau(F_i)\times \min_{F_j\subset F_i;|F_j|=|F_i|-1}m(F_j) \times |F_i|+m(F_i),$$ and $$m'(F_j)=m(F_j)+\tau(F_i)\times \min_{F_k\subset F_i;|F_k|=|F_k|-1}m(F_k),$$ when $F_j\subset F_i$ and $|F_j|=|F_i|-1$. Since the $\tau(F_i)\in[-1,0)$, $m'$ satisfies that $m'(F_i)\in[0,1]$ for $F_i\subseteq \Omega$. In addition
        $$\frac{\Delta m'(F_j)}{\Delta m'(F_i)}=\frac{\tau(F_i)\times \min_{F_k\subset F_i;|F_k|=|F_k|-1}m(F_k)}{\tau(F_i)\times \min_{F_j\subset F_i;|F_j|=|F_i|-1}m(F_j) \times |F_i|}=\frac{1}{|F_i|},$$ 
    and the number of $F_j$ is $|F_i|$, so $m'$ satisfies $\sum_{F_i\subseteq \Omega}m(F_i)=1$.
\end{proof}

\subsection{Proposition \ref{p5}}
\begin{proposition}[Transmittability]\label{p5}
    Consider two isopignistic transformations, $\mathfrak{IB}_1=\{\mathcal{G}_{\Omega},\boldsymbol{\zeta}_1\}$ and $\mathfrak{IB}_2=\{\mathcal{G}_{\Omega},\boldsymbol{\zeta}_2\}$, they satisfy $m_2=T_{\mathfrak{IB}_1}(m_1)$ and $m_3=T_{\mathfrak{IB}_2}(m_2)$. The transformation from $m_1$ to $m_3$ can be written as $m_3=T_{\mathfrak{IB}_{1+2}}(m_1)$, where $\mathfrak{IB}_{1+2}=\{\mathcal{G}_{\Omega},\zeta_{1}+\zeta_{2}\}$.
\end{proposition}

\begin{proof}
For the subset $F_i$, performing the transformation via $\mathfrak{IB}_1$ and $\mathfrak{IB}_2$ can achieve the following outcome
$$m_3(F_i)=m_1(F_i)-\zeta_1(F_i)+\sum_{F_i\subset F_k, |F_k|=|F_i|+1}\frac{\zeta_1(F_k)}{|F_k|}-\zeta_2(F_i)+\sum_{F_i\subset F_k, |F_k|=|F_i|+1}\frac{\zeta_2(F_k)}{|F_k|},$$ and performing the transformation via $\mathfrak{IB}_{1+2}$ can achieve the following outcome
$$m_{3}'=m_1(F_i)-(\zeta_1(F_i)+\zeta_2(F_i))+(\sum_{F_i\subset F_k, |F_k|=|F_i|+1}\frac{\zeta_1(F_k)+\zeta_2(F_k)}{|F_k|}).$$
It is evident that $m_3(F_i)=m_{3}'(F_i)$, and the isotransformation function satisfies transmittability.
\end{proof}

\subsection{Proposition \ref{p6}}

\begin{proposition}[Ergodicity]\label{p6}
Consider a $m$ under the frame $\Omega$, for arbitrary BPA $m'$ satisfying $m'\in \mathfrak{Iso}_{BetP_{m}}$, there must exist an isopignistic transformation with $\mathfrak{IB}=\{\mathcal{G}_{\Omega},\zeta\}$ satisfying $m'=T_{\mathfrak{IB}}(m)$.
\end{proposition}

\begin{proof}
    Since the original $m$ and the target $m'$ are in the identical isopignistic domain, they have equal $BetP$s. According to the Proposition \ref{p2}, they can be transformed to $BetP$ through $\mathfrak{IB}_{m}=\{\mathcal{G}_{\Omega},{\zeta}_{m}\}$, and $\mathfrak{IB}_{m'}=\{\mathcal{G}_{\Omega},{\zeta}_{m'}\}$. Based on the Proposition \ref{p3}, the transformation from $m'$ to $BetP$ can be realized via $\mathfrak{IB}^{-1}_{m'}=\{\mathcal{G}_{\Omega},-{\zeta}_{m'}\}$. Based on the Proposition \ref{p5}, the revision from $m$ to $m'$ can be implemented via $\mathfrak{IB}=\{\mathcal{G}_{\Omega},{\zeta}_{m}-{\zeta}_{m'}\}$. Hence, the proposed isopignistic transformation can cover the whole isopignistic domain.
\end{proof}

\subsection{Proposition \ref{p7}}

\begin{proposition}[lower and upper bounds]\label{p7}
Consider a BPA $m$ under an $n$-element frame $\Omega$. The commitment component resulting from the isopignistic canonical decomposition has lower and upper bounds, which correspond to probability and possibility distribution, respectively. In terms of the isopignistic ratio, its upper bound satisfies $\forall |F_i|>1$, $Iso^{\tau}(F_i)=1$, and its lower bound satisfies $\forall |F_i|>1$, $Iso^{\tau}(F_i)\leq 0$. In terms of the isopignistic function, its upper bound satisfies $\forall |F_i|>1$, $Iso^{\zeta}=IT^{\zeta}(m_{\rm{c}}, BetP_m)$, and its lower bound satisfies  $\forall |F_i|>1$, $Iso^{\zeta}(F_i)=0$.
\end{proposition}

\begin{proof}
    For the upper bound, when $\forall |F_i| > 1$, $Iso^{\tau}(F_i) = 1$, the beliefs on the focal sets with multiple elements are transferred into singletons. Since the isopignistic transformation only revises the mass function within the isopignistic domain, the corresponding Bayesian mass function equals $BetP_m$. Hence, the upper bound isopignstic function is $Iso^{\zeta}=IT^{\zeta}(m_{\rm{c}}, BetP_m)$. For the lower bound, since the consonant mass function represents the least committed case in the isopignistic domain, when no beliefs are transferred to subsets with smaller cardinalities, i.e., $\forall |F_i| > 1$, $Iso^{\zeta}(F_i) = 0$, the lower bound is reached. For focal sets satisfying $|F_i| > 1$, when the isopignistic ratio $Iso^{\tau}(F_i) \in [-1,0)$, since there is only one focal set for each cardinality in a consonant mass function, the $d$ in Algorithm \ref{iso_rcd_inv_tau} must be $0$, making it identical to $Iso^{\zeta}(F_i) = 0$. Based on the above, the upper and lower bounds of the isopignistic canonical decomposition correspond to the probability and possibility distributions within their respective isopignistic domains.
\end{proof}

\subsection{Proposition \ref{p8}}

\begin{proposition}[Reversible construction]\label{p8}
    Consider a power set $2^\Omega$ of a frame $\Omega$, and a mapping $pc: 2^\Omega \rightarrow [-1, 1]$. If $pc$ satisfies the following requirements: $\forall |F_i| = 1$, $pc(F_i) \in [0,1]$; $\forall |F_i| > 1$, $pc(F_i) \in [-1,1]$; and $pc(\emptyset) = 1 - \max_{\omega \in \Omega} pc(\{\omega\})$, then it can be reconstructed as a BPA via $m = IsoCD^{-1}[\tau](pc)$.
\end{proposition}

\begin{proof}
    Since the $pc(F_i)\in[0,1]$ for $|F_i|=1$, the singletons of $pc$ can be seen as a possibility distribution $Poss$. Suppose a ratio $\tau(F_i)=pc(F_i)$ for $|F_i|>1$, the target information distribution $m$ can be implemented via $\tau$ and $m_\text{c}$, where $m_\text{c}$ is the consonant mass function of $Poss$. According to the Proposition \ref{p4}, $m$ adheres the definition of BPA. Hence, for the information distribution $pc$ satisfying the above requirements, it must can be reconstructed as a BPA.
\end{proof}

\subsection{Proposition \ref{p9}}

\begin{proposition}[Range of propensity specificity]\label{p9}
    Given a BPA $m$ under an $n$-element frame, its range of propensity specificity is $[\frac{1}{n},1]$. When subsets with equal cardinalities hold the same beliefs, the propensity specificity reaches the minimum value $\frac{1}{n}$. When $m$ satisfies $m(\{\omega\})=1$, the propensity specificity reaches the maximum value $1$.
\end{proposition}

\begin{proof}
For each cardinality, the contributions of each element for $BetP$ is equal, hence its $BetP$ is the uniform probability distribution. Their corresponding $Poss_m$ is $Poss_{m}(\omega_i)=1$ $\forall \omega_i\in\Omega$, which equals the minimum specificity distribution in possibilistic structure. Hence, when propositions of $m$ with equal cardinalities hold the same beliefs, it reaches the minimum value $\frac{1}{n}$. When $m$ is a deterministic event $m(\{\omega_i\})=1$, its $BetP_m$ and $Poss_m$ also denotes a deterministic event, which satisfies $Poss_m(\omega_i)=1$ and $Poss_m(\omega_j)=0$, $\forall \omega_j\in\Omega\setminus\{\omega_i\}$. Hence, the propensity specificity reaches the maximum value $1$. Based on the above, the range of propensity specificity holds $[\frac{1}{n},1]$.
\end{proof}

\subsection{Proposition \ref{p10}}

\begin{proposition}[Range of commitment specificity]\label{p10}
    Given a BPA $m$ under an $n$-element frame, its range of propensity specificity is $[0,1]$. When $m$ is consonant, the commitment specificity attains the minimum value $0$. When $m$ is Bayesian, the commitment specificity reaches the maximum value $1$. Notably, in the scenario where $m$ represents a deterministic event, commitment specificity becomes meaningless.
\end{proposition}

\begin{proof}
When $m$ is consonant, its $Iso^\zeta$s of multi-element subsets are $0$, the commitment specificity equals $0$. When $m$ is Bayesian, its isopignisitc function satisfies $Iso^\zeta(F_i)=\sum_{F_i\subseteq F_j}m_{\rm{c}}(F_j)$, where $|F_i|\geq 2$ and $m_{\rm{c}}$ is the consonant form in $m$'s isopignistic domain. Since there is at most one focal set under each cardinality in the consonant mass function,  $\sum_{|F_i|\geq 2}Iso^\zeta(F_i)=\sum_{F_j\subseteq\Omega}m_{\rm{c}}(F_j)\times(|F_j|-1)$. Hence, the commitment propensity of Bayesian mass function reaches the maximum value $1$. When $m(\{\omega_i\})=1$, its propensity specificity has reached the maximum value $1$, and its isopignisitc domain is $\mathfrak{Iso}_{\boldsymbol{p}}=\{m\}$. Since there is only has one information granule in the domain, it is meaningless to discuss its commitment specificity.
\end{proof}

\subsection{Proposition \ref{p11}}

\begin{proposition}[commutativity]\label{p11}
Exchanging the two BPAs will not affect the outcome of the fusion $m_1\circledsmall{$\rm{H}$}m_2$=$m_2\circledsmall{$\rm{H}$}m_1$.
\end{proposition}

\begin{proof}
    In terms of the propensity component, the t-norms and t-conorms satisfy the commutativity. In terms of the commitment component, the arithmetical average satisfies the commutativity. Hence, the hyper-cautious combination rules satisfy the commutativity.
\end{proof}

\subsection{Proposition \ref{p12}}

\begin{proposition}[quasi-associativity]\label{p12}
It does not satisfy the associativity, i.e., $m_1\circledsmall{$\rm{H}$}m_2\circledsmall{$\rm{H}$}m_3\neq m_1\circledsmall{$\rm{H}$}(m_2\circledsmall{$\rm{H}$}m_3)$. However, it holds quasi-associativity, i.e., it can provide a $k$ sources information fusion frame.
\end{proposition}

\begin{proof}
In the case of three BPAs, the fusion of commitment components can be written as $\frac{\frac{a+b}{2}+c}{2}$. However, this does not equal $\frac{\frac{b+c}{2}+a}{2}$, so they do not satisfy the associativity. In multi-source information fusion task, the combination rule can be extended as
    $$
    \begin{aligned}
        &m_1\circledsmall{$\rm{H}$}\cdots\circledsmall{$\rm{H}$} m_k:\\
        &Iso^{\tau}_{m_1}=IsoD[\tau](m_1),\cdots ,Iso^{\tau}_{m_k}=IsoD[\tau](m_k),\\
               & Iso^{\tau}_{m_1\circledtiny{$\rm{H}$}\cdots\circledtiny{$\rm{H}$}m_k}(F_i)=\begin{cases}
                    Iso^{\tau}_{m_1}(F_i) {\rm{H}}\cdots {\rm{H}} Iso^{\tau}_{m_k}(F_i) & |F_i|=1\\
                   \frac{Iso^{\tau}_{m_1}(F_i)+\cdots+Iso^{\tau}_{m_k}(F_i)}{k} & |F_i|\geq2,\\
                   1-K & F_i=\emptyset\\
                \end{cases}\\
            & m_1\circledsmall{$\rm{H}$}\cdots\circledsmall{$\rm{H}$} m_k=IsoD^{-1}[\tau]\left (Iso^{\tau}_{m_1\circledtiny{$\rm{H}$}\cdots\circledtiny{$\rm{H}$}m_k}\right ),
    \end{aligned}
$$
where  $K=1-\max_{\omega_i\in \Omega}\left (Iso^{\tau}_{m_1}(\{\omega_i\})\circledsmall{$\rm{H}$}\cdots\circledsmall{$\rm{H}$} Iso^{\tau}_{m_k}(\{\omega_i\})\right)$, and $k$ is the number of sources. Hence, they hold the quasi-associativity.
\end{proof}

\subsection{Proposition \ref{p13}}

\begin{proposition}[idempotency]\label{p13}
    For the minimum rule and maximum rule, they satisfy $m\circledsmall{$\top$}_{\boldsymbol{m}}/\circledsmall{$\bot$}_{\boldsymbol{m}}m=m$.
\end{proposition}

\begin{proof}
    In terms of the propensity component, the operators for $\circledsmall{$\top$}_{\boldsymbol{m}}$ and $\circledsmall{$\bot$}_{\boldsymbol{m}}$ are minimum t-norm and maximum t-conorm, so they satisfy ${Iso^{\tau}}_{m}(\{\omega_i\})\top_{\boldsymbol{m}}/\bot_{\boldsymbol{m}} {Iso^{\tau}}_{m}(\{\omega_i\})={Iso^{\tau}}_{m}(\{\omega_i\})$. In terms of the commitment component, the fusion can be written as $\frac{{Iso^{\tau}}_{m}(F_i)+{Iso^{\tau}}_{m}(F_i)}{2}={Iso^{\tau}}_{m}(F_i)$. Hence, the cautious rule and bold rule in hyper-cautious TBM holds idempotency.
\end{proof}

\subsection{Proposition \ref{p14}}

 \begin{proposition}[quasi-neural element]\label{p14}
    For the product rule and probabilistic rule, their quasi-neural elements are $m_\Omega$ and $m_\emptyset$, respectively, i.e., for $m\circledsmall{$\top$}_{\boldsymbol{p}}m_\Omega/ \circledsmall{$\bot$}_{\boldsymbol{p}}m_\emptyset=m'$, it satisfies $BetP_{m}=BetP_{m'}$, and $S_\textrm{c}(m')\leq S_\textrm{c}(m)$. Especially, when $m$ is consonant, it satisfies $m\circledsmall{$\top$}_{\boldsymbol{p}}m_\Omega/ \circledsmall{$\bot$}_{\boldsymbol{p}}m_\emptyset=m$.
\end{proposition}

\begin{proof}
    The isopignistic ratios of $m_\Omega$ and $m_\emptyset$ are
    $${Iso^\tau}_{m_\Omega}(F_i)=\begin{cases}
        1 & |F_i|=1\\
        0 & $\textrm{Others}$
    \end{cases},{Iso^\tau}_{m_\emptyset}(F_i)=\begin{cases}
        1 & |F_i|=\emptyset\\
        0 & $\textrm{Others}$.
    \end{cases}$$
    And the combination rule can be written as
 $$
            \begin{aligned}
            &Iso^{\tau}_{m}=IsoD[\tau](m),\\
               & Iso^{\tau}_{m\circledtiny{$\top$}_{\boldsymbol{p}} m_{\Omega}}(F_i)=\begin{cases}
                   \top_{\boldsymbol{p}}(Iso^{\tau}_{m}(F_i),1)=Iso^{\tau}_{m}(F_i) & |F_i|=1\\
                   \frac{1}{2}\times(Iso^{\tau}_{m}(F_i)+0)=\frac{1}{2}\times Iso^{\tau}_{m}(F_i) & |F_i|\geq2,\\
                   Iso^{\tau}_{m}(F_i) & F_i=\emptyset\\
                \end{cases}\\
            & m\circledsmall{$\top$}_{\boldsymbol{p}} m_{\Omega}=IsoD^{-1}[\tau]\left (Iso^{\tau}_{m\circledtiny{$\top$}_{\boldsymbol{p}} m_{\Omega}}\right ),
            \end{aligned}
$$    
and
 $$
            \begin{aligned}
            &Iso^{\tau}_{m}=IsoD[\tau](m),\\
               & Iso^{\tau}_{m\circledtiny{$\bot$}_{\boldsymbol{p}} m_{\Omega}}(F_i)=\begin{cases}
                   \bot_{\boldsymbol{p}}(Iso^{\tau}_{m}(F_i),0)=Iso^{\tau}_{m}(F_i) & |F_i|=1\\
                   \frac{1}{2}\times(Iso^{\tau}_{m}(F_i)+0)=\frac{1}{2}\times Iso^{\tau}_{m}(F_i) & |F_i|\geq2,\\
                   Iso^{\tau}_{m}(F_i) & F_i=\emptyset\\
                \end{cases}\\
            &m\circledsmall{$\bot$}_{\boldsymbol{p}} m_{\emptyset}=IsoD^{-1}[\tau]\left (Iso^{\tau}_{m\circledtiny{$\bot$}_{\boldsymbol{p}} m_{\emptyset}}\right ).
            \end{aligned}
$$ 
In terms of propensity component, it is evident that isopignistic functions remain unchanged, hence their results of PPT satisfy $BetP( m\circledsmall{$\top$}_{\boldsymbol{p}} m_{\Omega})=BetP( m\circledsmall{$\bot$}_{\boldsymbol{p}} m_{\emptyset})=BetP_m$. In terms of commitment component, the isopignistic functions are closer to $0$. From the perspective of commitment specificity, the fused results are closer to their least commtiment case in isopignistic domain, so they satisfiy $S_\textrm{c}(m')\leq S_\textrm{c}(m)$. In addition, when $m$ is consnonant, the $Iso^{\tau}_{m}(F_i)=0$ for $|F_i|\geq2$. Based on the above results, it holds $m\circledsmall{$\top$}_{\boldsymbol{p}} m_{\Omega}= m\circledsmall{$\bot$}_{\boldsymbol{p}} m_{\emptyset}=m$. Hence,  $m_\Omega$ and $m_\emptyset$ are quasi-neural elements in product rule and probabilistic rule in hyper-cautious TBM.

\end{proof}

\subsection{Proposition \ref{p15}}

\begin{proposition}[informative monotonicity]\label{p15}
    For the combination $m_1$\circledsmall{$\top$}$m_2$=$m$, their propensity components satisfy
    $Iso_{m_j}(\{\omega_i\})\geq Iso_{m}(\{\omega_i\})$, where $j=\{1,2\}$ and $\omega_i\in\Omega$. For the combination $m_1$\circledsmall{$\bot$}$m_2$=$m$, their propensity components satisfy $Iso_{m_j}(\{\omega_i\})\leq Iso_{m}(\{\omega_i\})$, where $j=\{1,2\}$ and $\omega_i\in\Omega$.
\end{proposition}

\begin{proof}
    Since the t-norms satisfy the result can dominate the original granules, and the t-conorms satisfy the original granules can dominate the result, it is evident that the hyper-cautious combination rules have a same property.
  
\end{proof}

\newpage
\section{Algorithms}
\subsection{Algorithm \ref{ben_a}: Belief evolution network}
\begin{algorithm}[htbp]
\caption{Belief revision via $\mathfrak{B}$: $m_\text{B}=T_{\mathfrak{B}}(m)$}
\label{ben_a}
\textbf{Input}: Original BPA $m$, BEN $\mathfrak{B}=\{{\mathcal{G}_{\Omega}, {\tau}, {\xi}}\}$\\
% \textbf{Parameter}: Optional list of parameters\\
\textbf{Output}: Revised BPA $m_{\rm{B}}$
\begin{algorithmic}[1] %[1] enables line numbers
\FOR{$t\leftarrow 1$ to $|\Omega|-1$}
\FOR{$F_i\subseteq \Omega;|F_i|=|\Omega|-t+1$}
\STATE $\zeta(F_i)\leftarrow \tau(F_i)\times m(F_i)$
\STATE $m(F_i)\leftarrow m(F_i) - \zeta(F_i)$\;
\FOR{$F_j\subset F_i;|F_j|=|F_i|-1$}
\STATE $m(F_j)\leftarrow m(F_j)+\xi(\frac{F_i}{F_j})\times \zeta(F_i)$\;
\ENDFOR
\ENDFOR
\ENDFOR
\STATE  $m_\text{B}\leftarrow m$\;
\STATE \textbf{return} $m_\text{B}$
\end{algorithmic}
\end{algorithm}
\newpage
\subsection{Algorithm \ref{iso_rcd}: Generations of isotransformation function and ratio}
\begin{algorithm}[htbp]
\caption{Isopignistic transformation: ${\tau}=IT^{\tau}(m_1,m_2)$, ${\zeta}=IT^{\zeta}(m_1,m_2)$}
\label{iso_rcd}
\textbf{Input}: Original BPA $m_1$, Outcome BPA $m_2$\\
% \textbf{Parameter}: Optional list of parameters\\
\textbf{Output}: Isotransformation function $\zeta$, Isotransformation ratio $\tau$
\begin{algorithmic}[1] %[1] enables line numbers
\STATE \textit{\%Forward transfers:}
\FOR{$t\leftarrow 1$ to $|\Omega|-1$}
\FOR{$F_i\subseteq \Omega;|F_i|=|\Omega|-t+1$}
\STATE $\zeta(F_i)\leftarrow m_1(F_i)-m_2(F_i)$
\IF{$\zeta(F_i)>0$}
\STATE $\tau(F_i)\leftarrow \frac{\zeta(F_i)}{m_1(F_i)}$
\STATE $m_1(F_i)\leftarrow m_2(F_i)$
\FOR{$F_j\subset F_i$; $|F_j|+1=|F_i|$}
\STATE $m_1(F_j)\leftarrow m_1(F_j)+\frac{\zeta(F_i)}{|F_i|}$
\ENDFOR
\ENDIF
\ENDFOR
\ENDFOR
\STATE \textit{\% Backward transfers:}
\FOR{$t\leftarrow 1$ to $|\Omega|-1$}
\FOR{$i\leftarrow 0$ to $2^{|\Omega|}-1$}
\IF{$|F_i|=t+1$ and $\zeta(F_i)<0$}
\STATE $\tau(F_i) \leftarrow \frac{\zeta(F_i)}{|F_i|\min_{|F_j|=|F_i|-1,F_j\subset F_i}m_1(F_j)}$
\STATE $m_1(F_i)\leftarrow m_2(F_i)$
\FOR{$F_j\subset F_i$ and $|F_j|=|F_i|-1$}
\STATE $m_1(F_j)\leftarrow m_1(F_j)+\frac{\zeta(F_i)}{|F_i|}$
\ENDFOR
\ENDIF
\ENDFOR
\ENDFOR
\STATE \textbf{return} $\zeta$, $\tau$
\end{algorithmic}
\end{algorithm}
\newpage

\subsection{Algorithm \ref{iso_rcd_inv_zeta}: Transformation from isopignistic function to BPA}

\begin{algorithm}[htbp]
\caption{Inverse isopignistic transformation: $m = IsoCD^{-1}[\zeta](Iso^\zeta)$}
\label{iso_rcd_inv_zeta}
\textbf{Input}: Isopignistic function $Iso^\zeta$\\
% \textbf{Parameter}: Optional list of parameters\\
\textbf{Output}: target mass function $m$
\begin{algorithmic}[1] %[1] enables line numbers
\IF{$|F_i|=1$ and $F_i\subseteq\Omega$}
\STATE $Poss \leftarrow Iso^{\zeta} $
\ENDIF
\STATE $m_{\rm{c}}(F_i)\leftarrow Poss(\omega(t))-Poss(\omega(t+1))$, $F_i=\{\omega(1)\cdots\omega(t)\}$
\STATE $m\leftarrow m_{\rm{c}}$
\FOR{$t\leftarrow 1$ to $|\Omega|-1$}
\FOR{$F_i\subseteq \Omega;|F_i|=|\Omega|-t+1$}
\STATE $m(F_i) \leftarrow m(F_i)-Iso^{\zeta}(F_i)$
\FOR{$F_j\subset F_i$ and $|F_j|=|F_i|-1$}
\STATE $m(F_j)\leftarrow m(F_j)+\frac{\zeta(F_i)}{|F_i|}$
\ENDFOR
\ENDFOR
\ENDFOR
\STATE \textbf{return} $m$
\end{algorithmic}
\end{algorithm}
\newpage
\subsection{Algorithm \ref{iso_rcd_inv_tau}: Transformation from isopignistic ratio to BPA}

\begin{algorithm}[htbp]
\caption{Inverse isopignistic transformation: $m = IsoCD^{-1}[\tau](Iso^\tau)$}
\label{iso_rcd_inv_tau}
\textbf{Input}: Isopignistic ratio $Iso^\tau$\\
% \textbf{Parameter}: Optional list of parameters\\
\textbf{Output}: target mass function $m$
\begin{algorithmic}[1] %[1] enables line numbers
\IF{$|F_i|=1$ and $F_i\subseteq\Omega$}
\STATE $Poss \leftarrow Iso^{\tau} $
\ENDIF
\STATE $m_{\rm{c}}(F_i)\leftarrow Poss(\omega(t))-Poss(\omega(t+1))$, $F_i=\{\omega(1)\cdots\omega(t)\}$
\STATE $m\leftarrow m_{\rm{c}}$
\STATE \textit{\%Forward transfers:}
\FOR{$t\leftarrow 1$ to $|\Omega|-1$}
\FOR{$F_i\subseteq \Omega;|F_i|=|\Omega|-t+1$}
\IF{$\tau(F_i)>$0}
\STATE $m(F_i) \leftarrow m(F_i)\times(1-Iso^{\tau}(F_i))$
\FOR{$F_j\subset F_i$ and $|F_j|=|F_i|-1$}
\STATE $m(F_j) \leftarrow m(F_j)+\frac{m(F_i)\times Iso^{\tau}(F_i)}{|F_i|}$
\ENDFOR
\ENDIF
\ENDFOR
\ENDFOR
\STATE \textit{\%Backward transfers:}
\FOR{$t\leftarrow 1$ to $|\Omega|-1$}
\FOR{$i\leftarrow 0$ to $2^{|\Omega|}-1$}
\IF{$|F_i|=t+1$ and $Iso^{\tau}(F_i)<0$}
\STATE $d\leftarrow\min_{|F_j|=t,F_j\subset F_i}m(F_j)$
\STATE $m(F_i)\leftarrow m(F_i)-d\times Iso^{\tau}(F_i) \times |F_i|$
\FOR{$F_j\subset F_i$ and $|F_j|=|F_i|-1$}
\STATE $m(F_j)\leftarrow m(F_j)+d\times Iso^{\tau}(F_i)$
\ENDFOR
\ENDIF
\ENDFOR
\ENDFOR
\STATE \textbf{return} $m$
\end{algorithmic}
\end{algorithm}
\newpage
\section{Examples}
\subsection{Example \ref{e1}}

\begin{example}\label{e1}

    Consider two BPAs 
    $${m}_1=\{0,0,0.4333,0.2333,0,0,0.2333,0.1\},~{m}_2=\{0,0.05,0.6,0,0.05,0,0,0.3\}.$$
    For the isopignistic transformation ${m}_1=T_\mathfrak{IB}({m}_2)$, the implementation process of isotransformation function $\zeta$ and ratio $\tau$ is outlined as follows
    \begin{enumerate}
        \item In terms of the forward transfers and the loop with $|F_i|=3$, $$\zeta(F_7)=0.3-0.1=0.2>0\rightarrow\tau(F_7)=\frac{2}{3}.$$ Based on the Line 7,  
           $$m_2=\{0,0.05,0.6,0.0667,0.05,0.0667,0.0667,0.1\}.$$
        \item In terms of the forward transfers and the loop with $|F_i|=2$, 
           $$\zeta(F_3)=\zeta(F_6)=0.0667-0.2333=-0.1667<0,$$
           $$\zeta(F_5)=0.0667-0=0.0667>0\rightarrow \tau(F_5)=1.$$
        Based on the Line 7,  
           $$m_2=\{0,0.0833,0.6,0.0667,0.0833,0,0.0667,0.1\}.$$
        \item In terms of the forward transfers and the loop with $|F_i|=2$, 
        
           $$\tau(F_3)=\frac{-0.1667}{2\times0.0833}=-1,~m_2=\{0,0,0.5167,0.2333,0.0833,0,0.0667,0.1\}$$
          $$\tau(F_6)=\frac{-0.1667}{2\times0.0833}=-1,~m_2=\{0,0,0.4333,0.2333,0,0,0.2333,0.1\}$$
    
        \item Since $m_2$ has transformed to $m_1$, the $\zeta$ and ${\tau}$ can be output as
       $$\tau:~\{\tau(F_3)=-1, \tau(F_5)=1, \tau(F_6)=-1, \tau(F_7)=\frac{2}{3}\},$$$$\zeta:~\{\zeta(F_3)=-\frac{0.5}{3}, \zeta(F_5)=\frac{0.2}{3}, \zeta(F_6)=-\frac{0.5}{3}, \zeta(F_7)=0.2\}.$$
    \end{enumerate}

\end{example}
\subsection{Example \ref{e2}}

\begin{example}\label{e2}
    Consider a BPA $m$ under a $4$-element frame, its beliefs represented on the lattice without empty set and isopignistic function and ratio are shown in the Figures \ref{e2f1} and \ref{e2f2}.
    \begin{figure}[htbp!]
    \centering
    \includegraphics[width=0.65\textwidth]{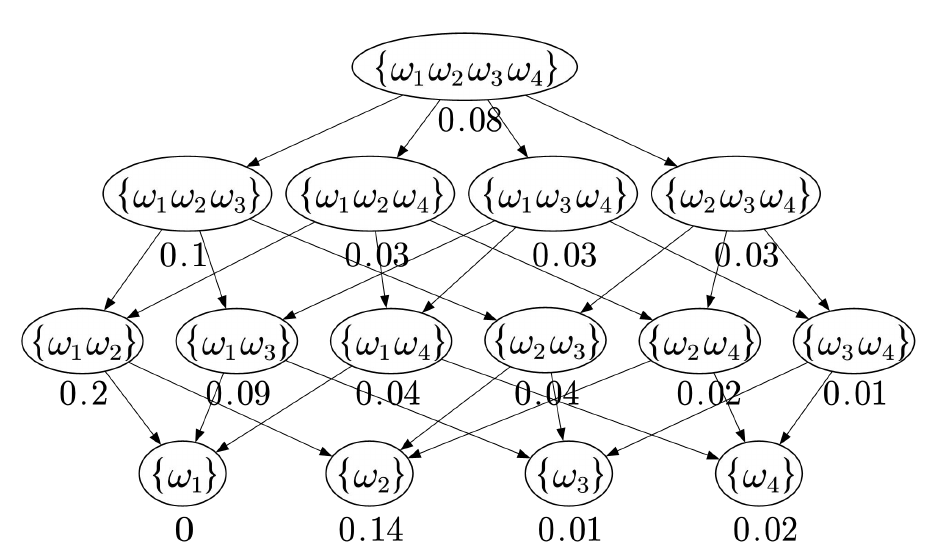}
    \caption{Representation of $m$ on belief structure}
    \label{e2f1}
\end{figure}
\begin{figure}[htbp!]
    \centering
    \includegraphics[width=0.65\textwidth]{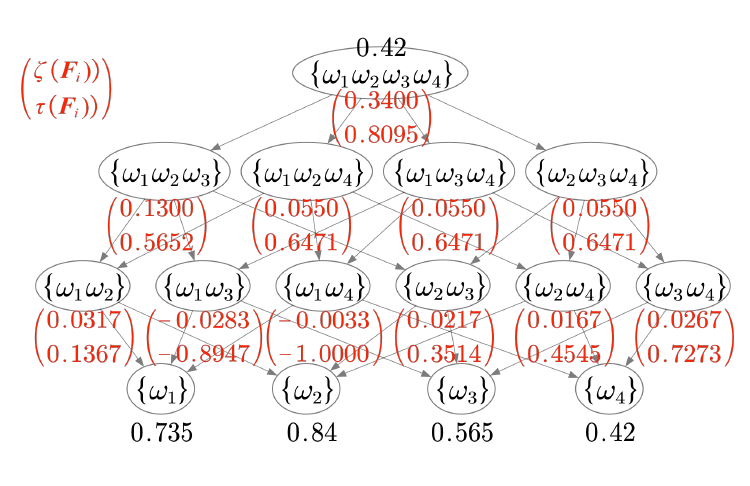}
    \caption{Isopignistic function and ratio of $m$}
    \label{e2f2}
\end{figure}
\end{example}
\subsection{Example \ref{e3}}
\begin{example}\label{e3}
    Under a 4-element frame $\Omega$, the values of singletons in $pc$ form a possibility distribution $\{1, 1, 1, 1\}$, and the values of multi-element subsets in $pc$ are given by:
        $$pc(F_{6})=0.5,pc(F_{12})=0.5,pc(F_{15})=0.5.$$
    Its isopignistic function can be implemented via $$IsoCD^{-1}[\zeta](IsoCD[\tau](pc))\rightarrow Iso^{\zeta}(F_{15})=0.5$$. Hence the corresponding BPA is 
        $$m(F_{15})=0.5,m(F_i)=0.125, |F_i|=3.$$
    Its isopignistic ratio can be implemented via $$IsoCD^{-1}[\tau](IsoCD[\tau](pc))\rightarrow Iso^{\tau}(F_{15})=0.5.$$
\end{example}

\subsection{Example \ref{e4}}

\begin{example}\label{e4}
    Given a BPA $$m=\{0,0.3,0.2,0,0,0.1,0.2,0.2\},$$ decompose $m$ via isopignistic canonical decomposition, Pichon's canonical decomposition, and Smets' canonical decomposition, respectively, their results are
    $$\begin{aligned}
        &Iso^{\zeta}=\{0,1,0.95,0.45,0.65,0.05,-0.05,0.45\},\\
        &Iso^{\tau}=\{0,1,0.95,1,0.65,0.3333,-1,0.6923\},\\
        & t=\{1,0.6,0.6,-0.16,0.5,0,0.1,0.04\},\\
        &\sigma=\{1.5,0.5,0.6667,1,1.2,0.6667,0.5\}.
    \end{aligned}$$
   When the values of the multi-element subsets vary within certain ranges, the corresponding mass functions will also vary, provided the normalization condition is maintained. According to the interpretation of the functions, the range of values adjusted for $iso^{\tau}$ and $t$ is $[-1,1]$, while the range of values adjusted for $\sigma$ is $[0,2]$. Variations of the mass functions are shown in Figure \ref{compare}.
\begin{figure}[htbp!]
    \centering
    \includegraphics[width=0.75\textwidth]{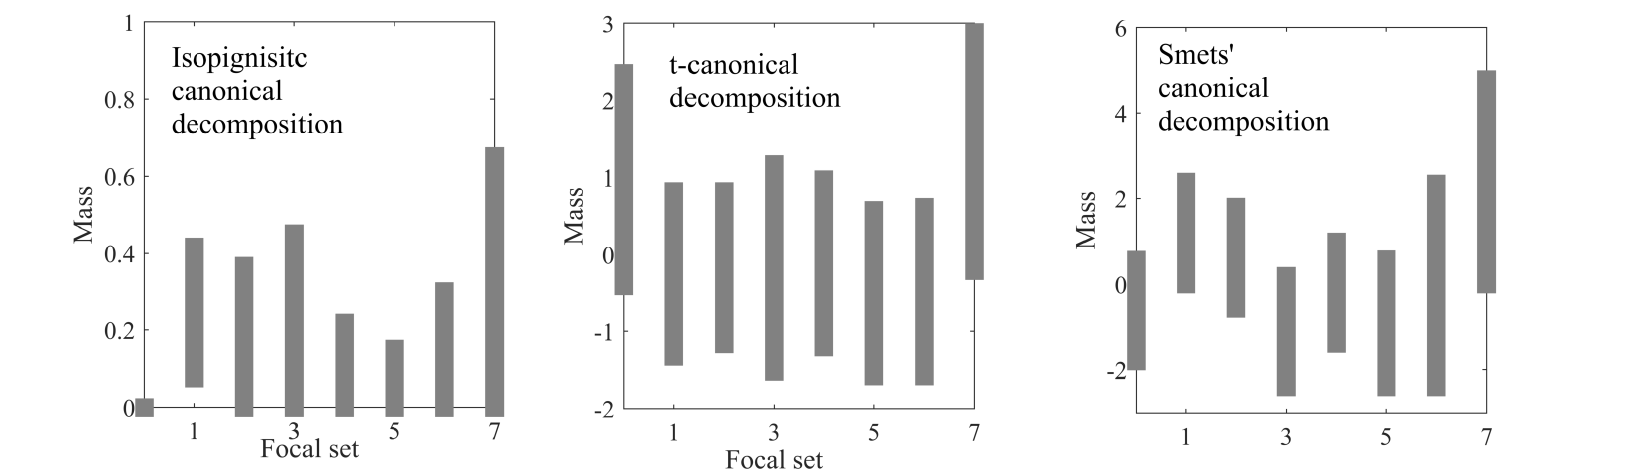}
    \caption{Variations of mass functions}
    \label{compare}
\end{figure}

\end{example}

\subsection{Example \ref{e5}}

\begin{example}\label{e5}
    Under a $3$-element frame, some BPAs and their isopignistic functions are shown in the Table \ref{e4t}. Their $BetP$s, Yager's specificity, propensity specificity, and commitment specificity are shown in the Table \ref{e4t2}.

    \begin{table}[htbp!]
        \centering
        \caption{BPAs and their isopignistic function in Example \ref{e4}}
        \label{e4t}
        \begin{tabular}{c|c||c|c}
        \Xhline{1pt}
           $m_1$ & $\{0,0.3333,0.3333,0,0.3333,0,0,0\} $&
            $Iso^{\zeta}_{m_1}$ & $\{0,1,1,0.3333,1,0.3333,0.3333,1\} $ \\
            \hline
            $m_2$ & $\{0,0,0,0,0,0,0,1\} $&
            $Iso^{\zeta}_{m_2}$ & $\{0,1,1,0,1,0,0,0\} $ \\
            \hline
            $m_3$ & $\{0,0,0,0.3333,0,0.3333,0.3333,0\} $&
            $Iso^{\zeta}_{m_3}$ & $\{0,1,1,0,1,0,0,1\} $ \\
            \hline
            $m_4$ & $\{0,0.4,0,0,0,0,0,0.6\} $&
            $Iso^{\zeta}_{m_4}$ & $\{0,1,0.6,0,0.6,0,0,0\} $ \\
             \hline
            $m_5$ & $\{0,0.5,0,0,0,0,0.2,0.3\} $&
            $Iso^{\zeta}_{m_5}$ & $\{0,1,0.6,0.2,0.6,0.2,-0.2,0.3\} $ \\
             \hline
            $m_6$ & $\{0,0,0,0.4,0,0,0,0.6\} $&
            $Iso^{\zeta}_{m_6}$ & $\{0,1,1,0,0.6,0,0,0\} $ \\
            \hline
            $m_7$ & $\{0,0,0,0.2,0,0,0.2,0.6\} $&
            $Iso^{\zeta}_{m_7}$ & $\{0,0.9,1,-0.1,0.9,0.1,-0.1,0.3\} $ \\
            \Xhline{1pt}
        \end{tabular}
        
    \end{table}

\begin{table}[htbp!]
        \centering
        \caption{$BetP$s and specificity measures in Example \ref{e4}}
        \label{e4t2}
        \begin{tabular}{c|c|c|c|c}
        \Xhline{1pt}
           $m$ & $BetP$ & $S$ & $S_{\rm{p}}$  &$S_{\rm{c}}$\\
           \hline
           $m_1$ & $\{0.3333,0.3333,0.3333\}$ & $1$ & $0.3333$ & $1$ \\
           \hline
           $m_2$ & $\{0.3333,0.3333,0.3333\}$ & $0.3333$ & $0.3333$ & $0$ \\
           \hline
           $m_3$ & $\{0.3333,0.3333,0.3333\}$ & $0.5$ & $0.3333$ & $0.5$ \\
           \hline
           $m_4$ & $\{0.6,0.2,0.2\}$ & $0.6$ & $0.6$ & $0$ \\
           \hline
           $m_5$ & $\{0.6,0.2,0.2\}$ & $0.7$ & $0.6$ & $0.3333$ \\
           \hline
           $m_6$ &$\{0.4,0.4,0.2\}$ & $0.4$ & $0.4$ & $0$ \\
           \hline
           $m_7$ & $\{0.3,0.4,0.3\}$ & $0.4$ & $0.4$ & $0.1111$ \\
            \Xhline{1pt}
        \end{tabular}
        
    \end{table}
    In Table \ref{e4t2}, $m_1$, $m_2$ and $m_3$ correspond to different values of $S$. Based on their $BetP$s, there is no difference in restricting the value of uncertain variable $X$. In terms of the proposed methods, their $S_{\rm{p}}$s reach the minimum value $\frac{1}{3}$, and $S_{\rm{c}}$s indicate that they are different in describing the specificity of the focal set. Thus, while Yager's method can distinguish between these three BPAs, utilizing specificity measures based on the isopignistic function can better elucidate the source of their distinction. It is obvious that $m_5$ is more specific than $m_4$, but their $S_{\rm{p}}$s are same, and $S_{\rm{c}}$s indicate that $m_5$ is more specific than $m_4$. Hence, specificity's difference of $m_4$ and $m_5$ is caused by the commitment's difference in isopignistic domain. For $m_6$ and $m_7$, though $S(m_6)=S(m_7)$, $S_{\rm{p}}(m_6)=S_{\rm{p}}(m_7)$ an $S_{\rm{p}}(m_6)<S_{\rm{p}}(m_7)$, it can not conclude that $m_7$ is more specific than $m_6$. Since they don't exist in an isopignistic domain, comparing commitment specificity is meaningless. 
\end{example}

\subsection{Example \ref{e6}}

\begin{example}\label{e6}
Given two BPAs under a $3$-element frame,
$$ m_1=\{0.02,0.1,0.1,0.25,0.06,0.27,0.02,0.18\}, m_2=\{0.07,0.05,0.16,0.21,0.14,0.31,0.05,0.01\}.$$
Fuse them via the diffidence function-based combination rules and the hyper-cautious combination rules, the results of them are shown in Table \ref{ecr1t}.
\begin{table}[htbp!]
    \centering
     \caption{Fusion results of $m_1$ and $m_2$ in Example \ref{e6}}
    \label{ecr1t}
    \begin{tabular}{c|cccccccc}
    \Xhline{1pt}
        Rule & $\emptyset$ & $\{\omega_1\}$ & $\{\omega_2\}$ & $\{\omega_1\omega_2\}$ & $\{\omega_3\}$ & $\{\omega_1\omega_3\}$ & $\{\omega_2\omega_3\}$ & $\{\omega_1\omega_2\omega_3\}$ \\
        \Xhline{1pt}
        \circledsmall{$\cap$} & $0.2780$&$0.2272$&$0.1317$&$0.0928$&$0.1161$&$0.1422$&$0.0102$&$0.0018$\\
        \hline
        $\circledsmall{$\top$}_{\boldsymbol{p}}$ & $0.0984$ & $0.1547$ & $0.1131$ & $0.1919$ & $0.0803$ & $0.2445$ & $0.0293$ & $0.0879$\\
        \hline
        \circledsmall{$\cup$} &$0.0014$ & $0.0130$ & $0.0262$ & $0.1897$ & $0.0154$ & $0.2267$ & $0.0410$ & $0.4866$\\
        \hline
        $\circledsmall{$\bot$}_{\boldsymbol{p}}$ & $0.0016$ & $0.0314$ & $0.1488$ & $0.2406$ & $0.1195$ & $0.3023$ & $0.0390$ & $0.1168$\\
        \hline
        \circledsmall{$\wedge$} & $0.9356$ & $0.0370$ & $0.0098$ & $0.0016$ & $0.0131$ & $0.0024$ & $0.0004$ & $0.0001$\\
        \hline
        $\circledsmall{$\top$}_{\boldsymbol{m}}$ & $0.0800$ & $0.0764$ & $0.1254$ & $0.2447$ & $0.0880$ & $0.2595$ & $0.0315$ & $0.0945$\\
        \hline
        \circledsmall{$\vee$} & $0.0043$ & $0.0213$ & $0.0213$ & $0.1437$ & $0.0128$ & $0.1235$ & $0.0239$ & $0.6494$\\
        \hline
         $\circledsmall{$\bot$}_{\boldsymbol{m}}$ & $0.0200$ & $0.0611$ & $0.1333$ & $0.2155$ & $0.1014$ & $0.3292$ & $0.0349$ & $0.1046$\\
        \Xhline{1pt}
    \end{tabular}
    \end{table}
    In addition, their $BetPs$ and corresponding Shannon entropies are shown in \ref{tab:ex2}.
    \begin{table}[htbp!]
          \centering
          \caption{$BetP$s of the fusion results and the order of beliefs.}
        \label{tab:ex2}
        \begin{tabular}{c|ccc|c|c}
        \hline
        Rule & $\omega_1$  & $\omega_2$  & $\omega_3$ & Order & Entropy\\
        \hline
            \circledsmall{$\cap$}  & $0.4783$ & $0.2546$ & $0.2672$ & $\omega_1\succ\omega_3\succ \omega_2$ & $1.5202$ \\
           \hline
              $\circledsmall{$\top$}_{\boldsymbol{p}}$& $0.4461$ & $0.2806$ & $0.2733$ & $\omega_1\succ\omega_2\succ \omega_3$ & $1.5454$ \\
           \hline
         
            \circledsmall{$\cup$}   & $0.3839$ & $0.3042$ & $0.3119$ & $\omega_1\succ\omega_3\succ \omega_2$ & $1.5768$\\
            \hline
           $\circledsmall{$\bot$}_{\boldsymbol{p}}$   & $0.3424$ & $0.3281$ & $0.3296$ & $\omega_1\succ\omega_3\succ \omega_2$ & $1.5874$ \\
           \hline
            
           \circledsmall{$\wedge$}  & $0.6061$ & $0.1686$ & $0.2253$ & $\omega_1\succ\omega_3\succ \omega_2$  & $1.3553$\\
           \hline
        $\circledsmall{$\top$}_{\boldsymbol{m}}$     & $0.3913$ & $0.3207$ & $0.2880$ & $\omega_1\succ\omega_2\succ \omega_3$ & $1.5731$ \\
           \hline
        
            \circledsmall{$\vee$} & $0.3729$ & $0.3229$ & $0.3042$& $\omega_1\succ\omega_2\succ \omega_3$ & $1.5796$ \\
           \hline
         $\circledsmall{$\bot$}_{\boldsymbol{m}}$    & $0.3759$ & $0.2993$ & $0.3248$ & $\omega_1\succ\omega_3\succ \omega_2$  & $1.5784$ \\
           \hline
        \end{tabular}  
    \end{table}
     In terms of the orders of the results, the hyper-cautious rules get the same order for the conjunctive rules and the disjunctive rules, respectively. In diffidence function-based rules, based on the information ordering, since bold rule is available in the credible and dependent sources, so its tendency of the decision outcome should less than the cautious rule and more than the disjunctive rule. However, bold rule leads the different result with other methods. In terms of the fusion results, the cautious rule and bold rule produce high beliefs on empty set and full set respectively, which seems do not match their ideal states of sources. 
\end{example}

% \bibliographystyle{alpha}
% \bibliography{sample}

\end{document}
